# Supplementary material for: Pedestrian flows through a narrow doorway: Effect of individual behaviours on the global flow and microscopic dynamics
Source: arXiv:1610.05909 source file (2017-01-09)
Supplement: Supplementary file 1 [file Supplementary_Information.pdf]

# Supplementary Information of "Pedestrian flows through a narrow doorway: effect of individual behaviours on the global flow and microscopic dynamics"

**Alexandre NICOLAS[1,2] and Sebastián BOUZAT[2] and Marcelo N. KUPERMAN[2]**

[1] LPTMS, CNRS & Univ. Paris-Sud, F-91405 Orsay, France
[2] CONICET & Centro Atómico Bariloche, Bariloche, 8400, Argentina

## Content

This supplemental section contains 7 figures and their captions in support of some statements made in the main text. It also provides additional information regarding the time-dependent flow rate and density fluctuations, along with the derivation of the relation between the mean time lapse between egresses and the mean dwell time in the exit zone. Also included as supplemental material are parts of the videos for the evacuations

- with placid walkers at an effective concentration of selfish participants $c_s^\star = 45\%$ ('evacuation_placid_cs=45pc.mp4'),
- with purposeful walkers at $c_s^\star = 0\%$ ('evacuation_purposeful_cs=0pc.mp4'),
- with purposeful walkers at $c_s^\star = 92\%$ ('evacuation_purposeful_cs=92pc.mp4'),
- with purposeful walkers at $c_s^\star = 100\%$ ('evacuation_purposeful_cs=100pc.mp4').

Note that the quality of the videos has deliberately been lowered very substantially, in order not to impinge on the participants' privacy. The rest of the primary data is available upon request to the authors.

## Video analysis

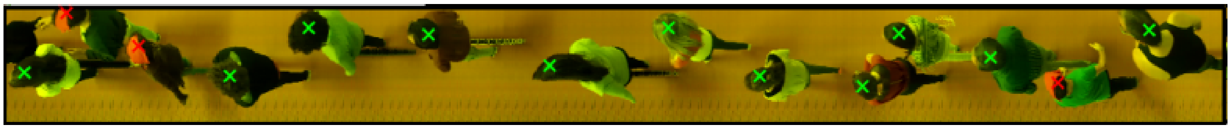

**Figure S1** Portion of the time line of pedestrians' egresses corresponding to the experiment with placid walkers at $c_s^\star = 45\%$. The red and green crosses were obtained by manually clicking on the pedestrians' heads.

## Density and flow rate fluctuations

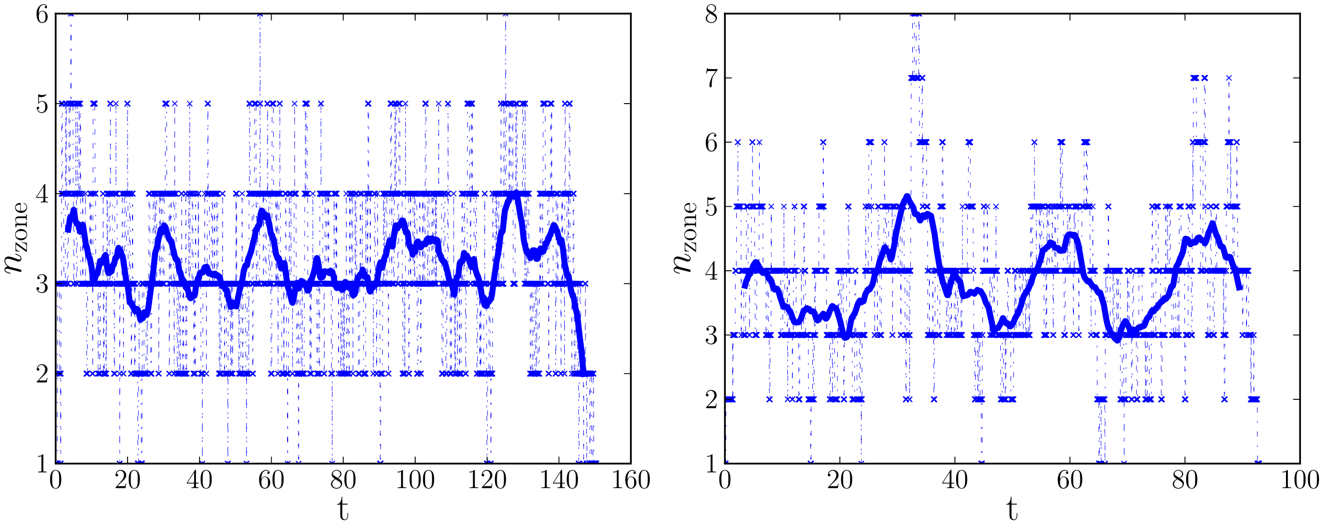


**Figure S2** (Thin dashed lines with crosses) Instantaneous number of pedestrians (occupancy) in the exit zone as a function of time, for the evacuations with (left) $c_s^\star = 71\%$(purposeful) and (right) $c_s^\star = 100\%$(purposeful). Also represented, with a thicker line, are the moving averages of the occupancy over time intervals $\delta t = 7\,\text{s}$. Note that, besides its fluctuations, the density is macroscopically not far from stationary, although a slight tendency to decrease with time is observed in some experiments, not unlike what is shown in Ref. [1]. On the right panel, corresponding to $c_s^\star = 100\%$, some oscillations with time are seen, which are potentially related to the re-injection scheme.

## Angles of incidence

## Dwell time (or waiting time) in the exit zone

### Relation with the mean time lapse

The distribution of time lapses $\Delta t$ between successive egresses provides information regarding the time series of passages through the door, whereas the distribution of dwell times $T_w$ in the exit zone offers a pedestrian-based perspective and its computation requires to keep track of the pedestrians from their entrance into the zone to to their egress. Notwithstanding this contrast, the mean values of these distributions are related by the simple relation $\langle T_w \rangle = \langle \rho \rangle A \langle \Delta t \rangle$, where $A$ is the area of the exit zone and $\rho$ is the pedestrian density.

Indeed, for an evacuation starting at $t = 0$ and ending at $t = T$, denoting $t_j^{\text{in}}$ and $t_j^{\text{out}}$ the times of entrance in, and egress from, the exit zone of pedestrian $j$, the average number of people $\langle \rho \rangle A$ in the exit zone can be expressed as

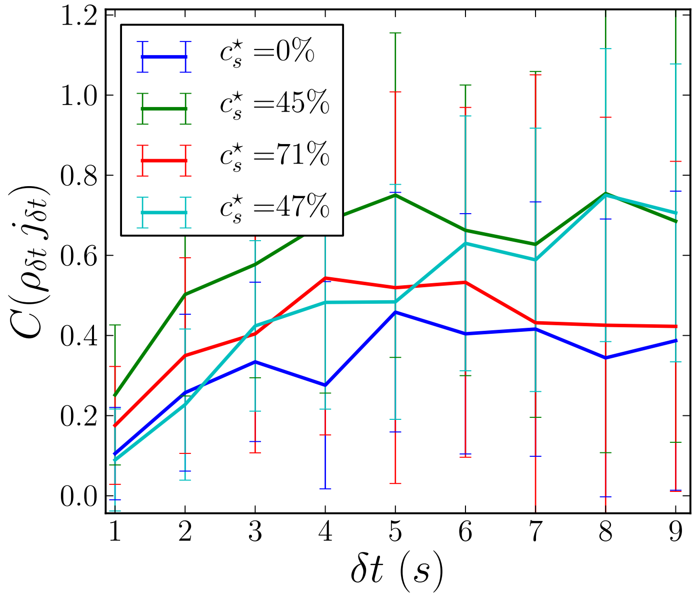


**Figure S3** Correlation function $C(\rho_{\delta t}, j_{\delta t})$ between the flow rate and density fluctuations in the placid experiments. The error bars represent an alleged 95% confidence interval (see *Error bars and confidence intervals* in the *Methods* of the main text).

$$\begin{aligned}\langle\rho\rangle A &= \frac{1}{T}\int_0^T \sum_{j=1}^{N}\left[\Theta\left(t-t_j^{\text{in}}\right)-\Theta\left(t-t_j^{\text{out}}\right)\right]\\ &= \frac{N}{T}\frac{1}{N}\sum_{j=1}^{N}\left(t_j^{\text{out}}-t_j^{\text{in}}\right)\\ &= J\,\langle T_w\rangle,\end{aligned}$$

where $\Theta$ is the Heaviside function, and provided that, for all pedestrians $j$, $0 \leqslant t_j^{\text{in}} \leqslant t_j^{\text{out}} \leqslant T$. It follows from $\langle\Delta t\rangle = J^{-1}$ that $\langle T_w\rangle = \langle\rho\rangle A\langle\Delta t\rangle$.

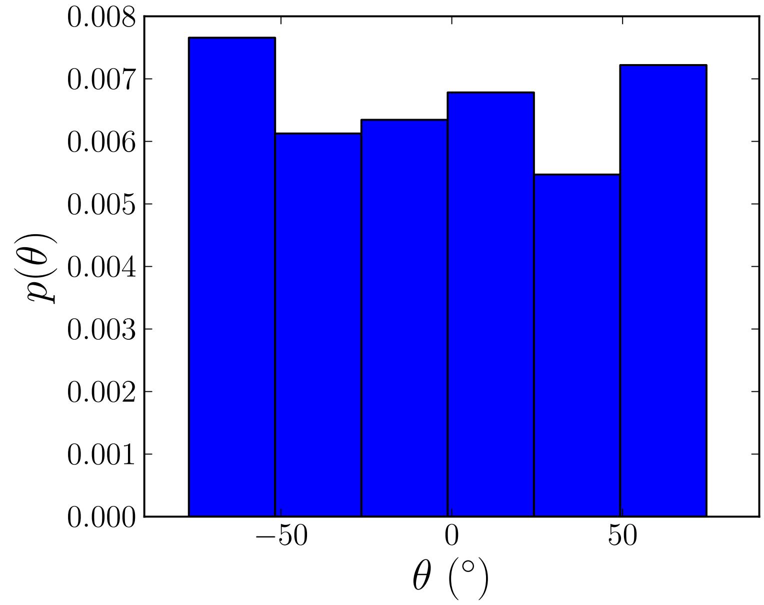


**Figure S4** Normalised histogram of the pedestrians' angles of incidence on the exit zone in the evacuation with purposeful walkers and a fraction $c_s^\star = 100\%$ of selfish agents.

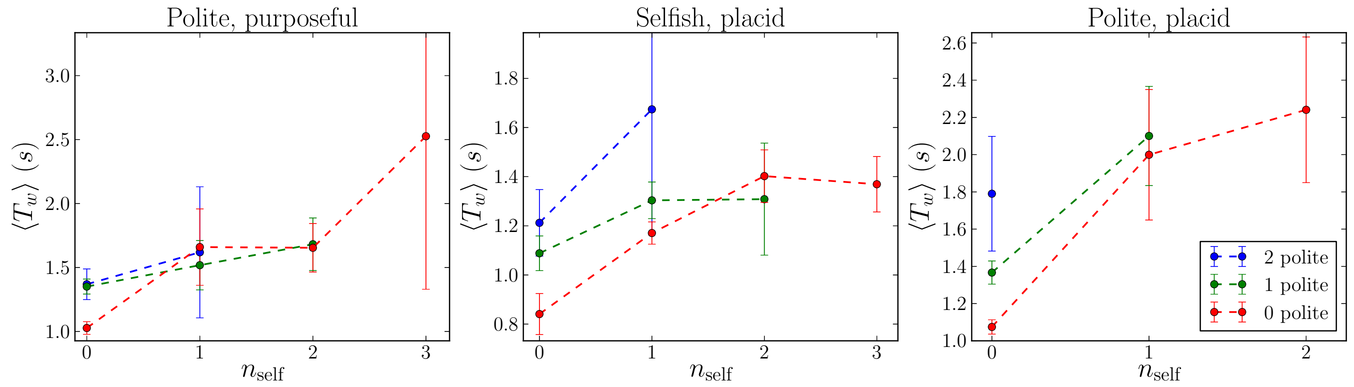


**Figure S5** Average dwell time in the exit zone of the pedestrian type indicated above the figure as a function of the number $n_{\mathrm{self}}$ of selfish participants in the zone, for distinct number of polite participants. The error bars represent an alleged 95% confidence interval (see *Error bars and confidence intervals* in the *Methods* of the main text).

# Disorder and perceived pressure

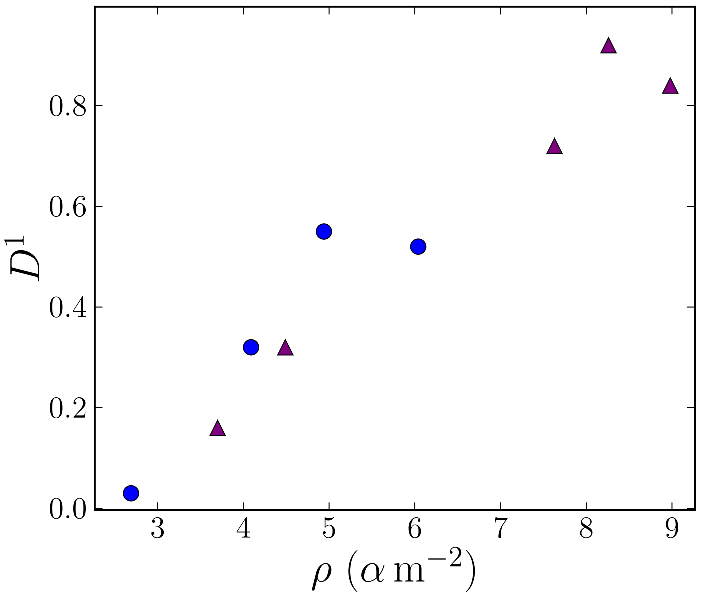


**Figure S6** Dependence on the density ρ of the disorder estimator $D^1 \equiv \frac{1}{N}\sum_{j=1}^{N}|k_{out}(j) - k_{in}(j)|$, where $k_{in}(j)$ and $k_{out}(j)$ are the order of entrance in the zone and egress of pedestrian $j$.

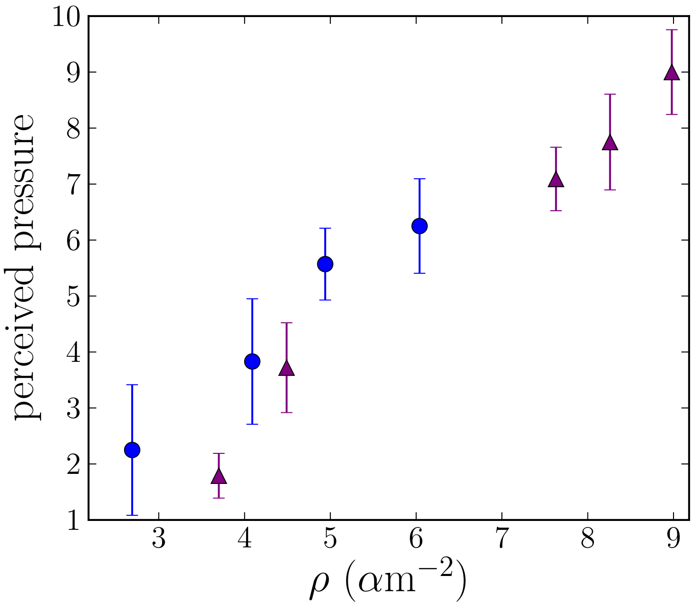


**Figure S7** Pressure felt by the participants as a function of the density at the door. The error bars represent an alleged 95% confidence interval (see *Error bars and confidence intervals* in the *Methods* of the main text). The order in which the evacuations were performed may have influenced the participants' perceptions; this may explain why the perceived pressure in e.g. the last experiment, at $c_s^\star = 0\%$(purposeful), is lower than that of the first experiment, at $c_s^\star = 0\%$(placid).

# References


[1] Simon Zens. Empirische Erfassung von Personenstromcharakteristika in Engstellen - Einfluss der Breite. Master's thesis, Bergische Universität Wuppertal, Wuppertal, Germany, 2008.
